# Supplementary material for: Modelling Electron Transfers Using Quasidiabatic Hartree-Fock States
Source: arXiv:1807.04983 ancillary file (2018-07-13)
Supplement: Supplementary file 1 [file supporting_info.pdf]

# Supporting Information

March 20, 2018

# 1 Stationary Point Geometries

## 1.1 C7H6F4

**Donor Equilibrium Geometry**
C1
C2 C1 1.43318378706
C3 C2 1.5490084942 C1 129.537343582
C4 C3 1.54958619497 C2 73.4995819491 C1 172.862954048
C5 C4 1.55937835552 C3 88.3968398167 C2 314.032064921
C6 C4 1.5495849471 C3 89.2882603856 C2 42.4475539609
C7 C4 1.48264749409 C3 126.181985878 C2 178.698802041
H1 C6 1.08754996395 C4 116.746505827 C3 68.1870668654
H2 C6 1.08671582849 C4 116.770214294 C3 205.042976751
F1 C1 1.23544313302 C2 123.035563007 C3 334.082975935
F2 C1 1.23544290952 C2 123.035556224 C3 157.343410002
H3 C3 1.08671546738 C2 117.107034685 C1 60.7708166755
H4 C3 1.08755024122 C2 115.439880618 C1 285.126368642
H5 C5 1.08675046126 C4 117.47712042 C3 154.419688645
H6 C5 1.08674980586 C4 117.476991203 C3 294.912356664
F3 C7 1.30872076336 C4 114.329919511 C3 54.4467751171
F4 C7 1.30872074483 C4 114.329971757 C3 184.498129126

**Minimum Energy Crossing Point**
C1
C2 C1 1.441
C3 C2 1.551 C1 127.098
C4 C3 1.551 C2 73.749 C1 179.5
C5 C4 1.585 C3 87.634 C2 314.7
C6 C4 1.551 C3 89.115 C2 42.4
C7 C4 1.441 C3 127.100 C2 180.5
H1 C6 1.088 C4 116.078 C3 69.2
H2 C6 1.087 C4 116.903 C3 205.2
F1 C1 1.268 C2 122.858 C3 328.1
F2 C1 1.268 C2 122.857 C3 155.1

H3 C3 1.087 C2 116.904 C1 67.1
H4 C3 1.088 C2 116.077 C1 291.0
H5 C5 1.087 C4 116.423 C3 155.7
H6 C5 1.087 C4 116.425 C3 293.5
F3 C7 1.268 C4 122.857 C3 31.9
F4 C7 1.268 C4 122.858 C3 204.9

**Acceptor Equilibrium Geometry**
C1
C2 C1 1.4826474239
C3 C2 1.54958619965 C1 126.182014725
C4 C3 1.54900827068 C2 73.4995906196 C1 181.301106514
C5 C4 1.59803492169 C3 87.0420514312 C2 315.39453688
C6 C4 1.54900768797 C3 89.3304664377 C2 42.4666276018
C7 C4 1.43318358858 C3 129.537411383 C2 187.137325733
H1 C6 1.0875498859 C4 115.439880892 C3 69.7967171831
H2 C6 1.0867157813 C4 117.107045568 C3 205.441231613
F1 C1 1.30872066873 C2 114.329838025 C3 305.552735209
F2 C1 1.30872068026 C2 114.329920389 C3 175.50157873
H3 C3 1.08671549938 C2 116.77025797 C1 68.7917024631
H4 C3 1.08755012874 C2 116.74657772 C1 291.935688829
H5 C5 1.08675052694 C4 115.362652575 C3 157.214660853
H6 C5 1.08674995884 C4 115.362691512 C3 292.266757395
F3 C7 1.23544318117 C4 123.035562179 C3 25.9165364637
F4 C7 1.23544301386 C4 123.03555679 C3 202.656075829

**Reference Structure for Surface Plots**
17

C 0.000000 0.000000 -2.371670
C -0.000000 0.000000 -0.930464
C 1.087948 -0.595812 -0.000019
C 0.000000 -0.000000 0.930464
C -0.000000 1.282830 0.000005
C -1.087936 -0.595836 0.000012
C 0.000000 0.000000 2.371672
H -1.175671 -1.680312 0.000009
H -2.057545 -0.105111 0.000029
F 0.000000 0.000000 -3.371670
F 0.000000 0.000000 -3.371670
H 2.057551 -0.105065 -0.000029
H 1.175693 -1.680288 -0.000027
H -0.907960 1.880358 0.000022
H 0.907957 1.880373 -0.000006
F 0.000000 0.000000 3.371672
F 0.000000 0.000000 3.371672

Structures for calculations were generated by changing the positions of F10, F11, and F16 and F17 interpolating between the following two sets of ($\angle CCF_1$, $\angle CCF_2$, $\angle$CCC, $r_{CF1}$, $r_{CF2}$, $r_{FF}$)

1. (123.2116, 123.2116, 113.5768, 1.2704, 1.2704, 2.1258)
2. (114.3100, 114.3101, 111.3757, 1.3087, 1.3087, 2.1619)

To generate the staggered structures, F16 and F17 were subsequently rotated 120 degrees about the z-axis.

## 1.2 Alizarin

**Donor Equilibrium Geometry**
C1
C2 C1 5.00262783915
C3 C2 2.49271829675 C1 2.42768629498
C4 C1 1.41409187558 C2 148.407874456 C3 214.655848166
C5 C2 1.39285065773 C1 149.429970456 C3 149.434286429
C6 C1 1.39655310266 C2 27.9037044343 C3 215.519284815
C7 C2 1.40485043305 C1 29.2174470419 C3 145.296113288
C8 C6 1.42759124706 C1 117.666239068 C2 182.165153673
C9 C7 1.41061880622 C2 119.496410326 C1 177.780879795
C10 C4 1.38422123905 C1 121.556585131 C2 359.309523324
C11 C5 1.40179913902 C2 120.190453959 C1 357.463573798
C12 C9 1.47593754502 C7 120.482314154 C2 179.693043539
C13 C10 1.39784567586 C4 118.549214446 C1 0.0711337632184
C14 C11 1.39247045654 C5 120.094826486 C2 0.0165156945059
Ti1 C4 2.74127377886 C1 76.4657071269 C2 179.894857136
O1 C1 1.32602985743 C2 98.7608664055 C3 34.7042346428
O2 C3 1.21564087263 C2 89.8653195692 C1 209.854970931
O3 C4 1.34291581298 C1 113.555373215 C2 178.935476706
O4 C12 1.21815050939 C9 120.19236653 C7 181.247709891
O5 Ti1 1.77749784708 C4 107.313166028 C1 96.9334772116
O6 Ti1 2.37504646883 C4 83.5430316755 C1 277.518746162
O7 Ti1 1.83883933664 C4 127.647805624 C1 215.563507974
O8 Ti1 2.19478704714 C4 129.219732243 C1 344.698356405
H1 C10 1.07424319399 C4 120.041162572 C1 180.343594186
H2 C11 1.07496604589 C5 120.043560375 C2 180.043811893
H3 C13 1.07205271719 C10 120.456227009 C4 180.454007129
H4 C14 1.07252923354 C11 120.993065486 C5 180.12824985
H5 O5 0.947607026493 Ti1 127.529481275 C4 345.605970058
H6 O6 0.952221495269 Ti1 101.245839225 C4 252.344151868
H7 O7 0.948871744108 Ti1 118.057083778 C4 246.162248739
H8 O6 0.950069307158 Ti1 114.923424924 C4 8.72814329703

H9 O8 0.951084949563 Ti1 112.032489517 C4 256.111323626
H10 O8 0.956849278044 Ti1 103.535540138 C4 12.1573429347
H11 C2 1.07230039161 C1 89.6528016155 C3 327.360988878
H12 C5 1.07501537913 C2 119.80387122 C1 177.476578112

**Minimum Energy Crossing Point**
0 1
C1
C2 C1 5.006
C3 C2 2.493 C1 1.966
C4 C1 1.427 C2 148.040 C3 201.9
C5 C2 1.393 C1 149.698 C3 159.8
C6 C1 1.403 C2 28.185 C3 203.3
C7 C2 1.405 C1 29.442 C3 157.4
C8 C6 1.427 C1 118.120 C2 181.5
C9 C7 1.411 C2 119.532 C1 178.7
C10 C4 1.403 C1 121.373 C2 0.6
C11 C5 1.402 C2 120.169 C1 358.6
C12 C9 1.475 C7 120.272 C2 179.8
C13 C10 1.388 C4 118.753 C1 359.7
C14 C11 1.393 C5 120.137 C2 359.9
Ti1 C4 2.794 C1 76.105 C2 181.4
O1 C1 1.308 C2 98.540 C3 21.8
O2 C3 1.216 C2 89.689 C1 200.1
O3 C4 1.305 C1 114.662 C2 180.0
O4 C12 1.220 C9 120.319 C7 180.7
O5 Ti1 1.820 C4 102.878 C1 95.9
O6 Ti1 2.339 C4 88.425 C1 280.2
O7 Ti1 1.857 C4 123.586 C1 211.7
O8 Ti1 2.219 C4 130.565 C1 353.7
H1 C10 1.075 C4 119.415 C1 180.0
H2 C11 1.076 C5 119.968 C2 180.0
H3 C13 1.072 C10 120.486 C4 180.4
H4 C14 1.073 C11 120.792 C5 180.0
H5 O5 0.947 Ti1 125.875 C4 11.3
H6 O6 0.953 Ti1 99.882 C4 249.6
H7 O7 0.948 Ti1 119.961 C4 246.7
H8 O6 0.950 Ti1 118.032 C4 7.4
H9 O8 0.952 Ti1 108.584 C4 283.4
H10 O8 0.956 Ti1 103.603 C4 35.7
H11 C2 1.072 C1 89.443 C3 338.5
H12 C5 1.075 C2 119.792 C1 178.6

**Acceptor Equilibrium Geometry**
C1
C2 C1 5.01123511676

C3 C2 2.49294483322 C1 1.72112253047
C4 C1 1.46505534486 C2 147.007908592 C3 165.341558664
C5 C2 1.39328304255 C1 149.730477253 C3 191.989622639
C6 C1 1.41202815646 C2 28.3688512607 C3 166.56465724
C7 C2 1.40508160882 C1 29.4888246181 C3 193.204400412
C8 C6 1.42295112863 C1 118.817085065 C2 179.624551672
C9 C7 1.41158663243 C2 119.376650291 C1 180.626784154
C10 C4 1.4426990494 C1 120.619252378 C2 1.91360876614
C11 C5 1.40248632965 C2 120.275367305 C1 0.748015226046
C12 C9 1.46709232065 C7 120.039024979 C2 180.138597026
C13 C10 1.36324680078 C4 119.160019558 C1 359.373562449
C14 C11 1.39224386622 C5 120.100508787 C2 0.00602653260207
Ti1 C4 2.95979225692 C1 74.5300553254 C2 185.164256512
O1 C1 1.27607770299 C2 98.4857627844 C3 345.504366234
O2 C3 1.21720976479 C2 89.6705512182 C1 168.182500806
O3 C4 1.23771324085 C1 117.40905355 C2 181.657445648
O4 C12 1.22598435471 C9 120.738429431 C7 179.855797416
O5 Ti1 1.91676940704 C4 94.1398872025 C1 96.1451337281
O6 Ti1 2.31326532705 C4 93.8368207657 C1 283.202497736
O7 Ti1 1.88628700664 C4 121.889645691 C1 209.987116228
O8 Ti1 2.20894231583 C4 128.438860769 C1 17.8224583037
H1 C10 1.07371030705 C4 118.109590053 C1 179.653985123
H2 C11 1.07477994706 C5 120.056501921 C2 179.964677353
H3 C13 1.07158141387 C10 120.938640914 C4 180.118313125
H4 C14 1.07260889918 C11 120.951221811 C5 179.920011201
H5 O5 0.944971388045 Ti1 125.063492596 C4 41.5580529806
H6 O6 0.953463180726 Ti1 99.4853036315 C4 244.914189786
H7 O7 0.945536580855 Ti1 124.057006031 C4 254.651321231
H8 O6 0.947685049973 Ti1 124.525400903 C4 6.70431425261
H9 O8 0.953847865667 Ti1 106.319473469 C4 334.484887724
H10 O8 0.957360648622 Ti1 95.5687756228 C4 84.0792970683
H11 C2 1.07216374462 C1 89.3761926201 C3 12.5692257847
H12 C5 1.07482996317 C2 119.758794423 C1 180.718073121

# 2 Electronic Energies of Stationary Points

## 2.1 C7H6F4

| Geometry | D | A | E | NOCI 1 | NOCI 2 | NOCI 3 |
|---|---|---|---|---|---|---|
| Donor | -665.920975 | N/A | N/A | N/A | N/A | N/A |
| MECP | -665.901250 | -665.901246 | -665.888360 | -665.9159 | -665.8761 | -665.4723 |
| Acceptor | N/A | -665.920975 | N/A | N/A | N/A | N/A |

## 2.2 Alizarin

### Donor Equilibrium Geometry

| SCF | 15-state NOCI | 3-state NOCI |
|---|---|---|
| -1984.6269015 | -1984.7008943 | -1984.6901613 |
| -1984.6184679 | -1984.5856879 | -1984.5827627 |
| -1984.6180286 | -1984.5658732 | -1984.5442076 |
| -1984.6154757 | -1984.5591412 | -1984.4409574 |
| -1984.6115577 | -1984.5568576 | -1984.3339795 |
| -1984.5536735 | -1984.5198503 | -1984.2481509 |
| -1984.4884403 | -1984.5192936 | |
| -1984.4874327 | -1984.4976822 | |
| -1984.4866775 | -1984.4850425 | |
| -1984.4825453 | -1984.4813869 | |
| -1984.4671158 | -1984.4517581 | |
| -1984.4484554 | -1984.4496776 | |
| -1984.4418763 | -1984.441352 | |
| -1984.4358894 | -1984.4395266 | |
| -1984.4187231 | -1984.423793 | |
| | -1984.4231528 | |
| | -1984.4079447 | |
| | -1984.4033419 | |
| | -1984.3957604 | |
| | -1984.3926122 | |
| | -1984.3854906 | |
| | -1984.3368457 | |
| | -1984.3090838 | |
| | -1984.2990742 | |
| | -1984.2337259 | |
| | -1984.1953352 | |
| | -1984.147044 | |
| | -1984.1109129 | |
| | -1983.6144182 | |
| | -1890.76896 | |

**Minimum Energy Crossing Point**

| SCF A | SCF D | SCF E | 3-state NOCI A | 3-state NOCI D | 6-state NOCI |
|---|---|---|---|---|---|
| -1984.6172103 | -1984.6172423 | -1984.6041564 | -1984.6549587 | -1984.6800595 | -1984.6906306 |
| -1984.6050068 | -1984.6090449 | -1984.5941169 | -1984.6405892 | -1984.573384 | -1984.6408262 |
| -1984.6035021 | -1984.6084872 | -1984.5918282 | -1984.5300737 | -1984.5366177 | -1984.6139136 |
| | | | -1984.5165646 | -1984.433813 | -1984.5737766 |
| | | | -1984.3170676 | -1984.3309373 | -1984.5369251 |
| | | | -1984.3091198 | -1984.241309 | -1984.5158126 |
| | | | | | -1984.4894041 |
| | | | | | -1984.4246533 |
| | | | | | -1984.3386595 |
| | | | | | -1984.309562 |
| | | | | | -1984.3031967 |
| | | | | | -1984.2329599 |

**Acceptor Equilibrium Geometry**

| SCF | 15-state NOCI | 3-state NOCI |
|---|---|---|
| -1984.6518460 | -1984.6942795 | -1984.6831367 |
| -1984.6392838 | -1984.6929805 | -1984.681843 |
| -1984.6379468 | -1984.6227898 | -1984.5581697 |
| -1984.6305883 | -1984.6225593 | -1984.5569365 |
| -1984.5841644 | -1984.6131504 | -1984.3445574 |
| -1984.5834581 | -1984.6131415 | -1984.3437684 |
| -1984.5729239 | -1984.5893965 | |
| -1984.5721891 | -1984.5886192 | |
| -1984.5712972 | -1984.5731069 | |
| -1984.5653107 | -1984.5730521 | |
| -1984.5626681 | -1984.5707915 | |
| -1984.5615428 | -1984.5707859 | |
| -1984.5614947 | -1984.5617448 | |
| -1984.5552570 | -1984.5617297 | |
| -1984.5552508 | -1984.537230 | |
| | -1984.5369743 | |
| | -1984.5050983 | |
| | -1984.5050296 | |
| | -1984.4658436 | |
| | -1984.4658104 | |
| | -1984.4515832 | |
| | -1984.4515783 | |
| | -1984.4292644 | |
| | -1984.4288199 | |
| | -1984.3329789 | |
| | -1984.3322057 | |
| | -1984.243802 | |
| | -1984.2437366 | |
| | -1983.8168644 | |
| | -1983.8159135 | |
